# Supplementary material for: Tunable Degenerate Optical Parametric Oscillation with Coupled Microresonators
Source: arXiv:2407.19129 source file (2024-07-27)
Supplement: Supplementary file 1 [file DOPO_photmolecule_SM.tex]

\documentclass[9pt]{osa-supplemental-document}
\setboolean{shortarticle}{false}

\usepackage{lineno}
\linenumbers % Turn off line numbering for Optica Open preprint submissions.

\usepackage{upgreek}
\usepackage[capitalise]{cleveref}
\usepackage{chemformula}
\usepackage{bigints}

\usepackage[textsize=footnotesize, 
tickmarkheight=5pt, 
color=blue!30, 
bordercolor=blue!30]{todonotes}

% \renewcommand{\thesection}{S\arabic{section}}
% \renewcommand{\thetable}{S\arabic\c@table}
% \renewcommand{\theequation}{S\arabic{equation}}
% \renewcommand{\thefigure}{S\arabic{figure}}
% \renewcommand{\bibnumfmt}[1]{[S#1]}
% \renewcommand{\citenumfont}[1]{S#1}

% \title{Title of primary manuscript: supplemental document}
\title{Dual-pumped degenerate optical parametric oscillators within triple-state photonic molecules: supplemental document}
\author{} %leave this blank
%% DO NOT ADD AUTHOR INFORMATION HERE; IT WILL BE ADDED DURING PRODUCTION

\setboolean{displaycopyright}{false} %copyright statement should not display in the  supplemental document

\begin{document}

\maketitle

\input{DOPO_body.tex}

\bibliography{DOPO_photmolecule.bib}
\end{document}
